# Supplementary material for: Enhancing the use of Galactic neutron stars as physical laboratories with precise astrometry
Source: arXiv:2212.08881 source file (2023-02-27)
Supplement: Supplementary file 1 [file appendixA.tex]

\chapter[Appendix A]{Authorship indication forms}

%\includepdf[pages=-]{authorship_forms/Ch3.pdf}

%\includegraphics[scale=0.75]{authorship_forms/Walter.png}

%\includepdf[pages=-]{authorship_forms/Ch4.pdf}

%\includepdf[pages=-]{authorship_forms/Ch5.pdf}

%\includepdf[pages=-]{authorship_forms/Ch6.pdf}

%\includepdf[pages=-]{authorship_forms/Ch7.pdf}

%\includepdf[pages=-]{authorship_forms/Ch8.pdf}

%\includepdf[pages=-]{authorship_forms/authorship_form_combined.pdf}
